# Supplementary material for: The Gelfand-Tsetlin Realisation of Simple Modules and Monomial Bases
Source: arXiv:1812.00976 source file (2018-12-03)
Supplement: Supplementary file 1 [file appendixA.tex]

\chapter{The Second Squared Chapter}

An average essay may contain five chapters, but I didn't plan my work properly
and then ran out of time. I spent too much time positioning my figures and worrying
about my preferred typographic style, rather than just using what was provided.
I wasted days bolding section headings and using double slash line endings, and 
had to remove them all again. I spent sleepless nights configuring manually numbered lists
to use the \LaTeX\ environments because I didn't use them from the start or understand
how to search and replace easily with texmaker.

Everyone has to take some shortcuts
at some point to meet deadlines. Time did not allow to test model 
B as well. So I'll skip right ahead and put that under my Future Work section.

\section{This is a section} 
Text text text text text text text text text text text text text text
text text text text text text text text text text text text text text
text text text text text text text text text text text text text text
text text text text text text text text text text text text text text
text text text text text. 

Some essays may have 3, 5 or 6 chapters. This is just an example. 
More importantly, do you have at most 35 pages?  
Luck has nothing to do with it. Use the techniques suggested for
writing your essay.

Now you're demonstrating pure talent and newly acquired skills. 
Perhaps some persistence. Definitely some inspiration. What was that about perspiration? 
Some team work helps, so every now and then why not browse your friends' essays and provide
some constructive feedback?
